# Supplementary material for: Measurements of ${}^3_\Lambda \rm{H}$ and ${}^4_\Lambda \rm{H}$ Lifetimes and Yields in Au+Au Collisions in the High Baryon Density Region
Source: arXiv:2110.09513 source file (2022-05-19)
Supplement: Supplementary file 1 [file supplementary.tex]

\RequirePackage{lineno}
\documentclass[floatfix,twocolumn,preprintnumbers,amsmath,amssymb,prl,superscriptaddress]{revtex4} 
\usepackage{url}
\usepackage{graphicx}% Includex figure files
\usepackage{dcolumn}% Align table columns on decimal point
\usepackage{xspace}
\usepackage{bm}% bold math
\usepackage{soul}
\usepackage{ulem}
\usepackage{xcolor}

\newcommand{\snn}{\mbox{$\sqrt{s_{\rm NN}}$}\xspace}
\newcommand{\hyt}{\mbox{${}^3_\Lambda \rm{H}$}\xspace}
\newcommand{\hyh}{\mbox{${}^4_\Lambda \rm{H}$}\xspace}
\usepackage{color}
\usepackage{natbib}
\widowpenalty=10000
\clubpenalty=10000
\begin{document}
%\linenumbers
\raggedbottom
\title{
Measurements of \hyt and \hyh Lifetime and Yield in Au+Au Collisions in the High Baryon Density Region: Supplementary Material
}

\input{star-author-list-2021-09-06.aps.tex}

\maketitle
%\begin{linenumbers}
\realpagewiselinenumbers
\setlength\linenumbersep{0.10cm}

\section{Additional information on the \hyt, \hyh lifetime analysis}
The main text describes the lifetime analysis using the \snn = 3.0\,GeV data set. The \snn = 7.2\,GeV analysis is similar, despite the difference in acceptance in the center-of-mass frame. Figure~\ref{fig:7p2acc} shows the $p_{T}$ as a function of $y$ for reconstructed \hyt and \hyh candidates using the \snn = 7.2\,GeV data set. The mid-rapidity region ($|y|<0.5$) is not covered for this data set. 

\begin{figure}[!htb]
\centering
\centerline{\includegraphics[width=0.5\textwidth]{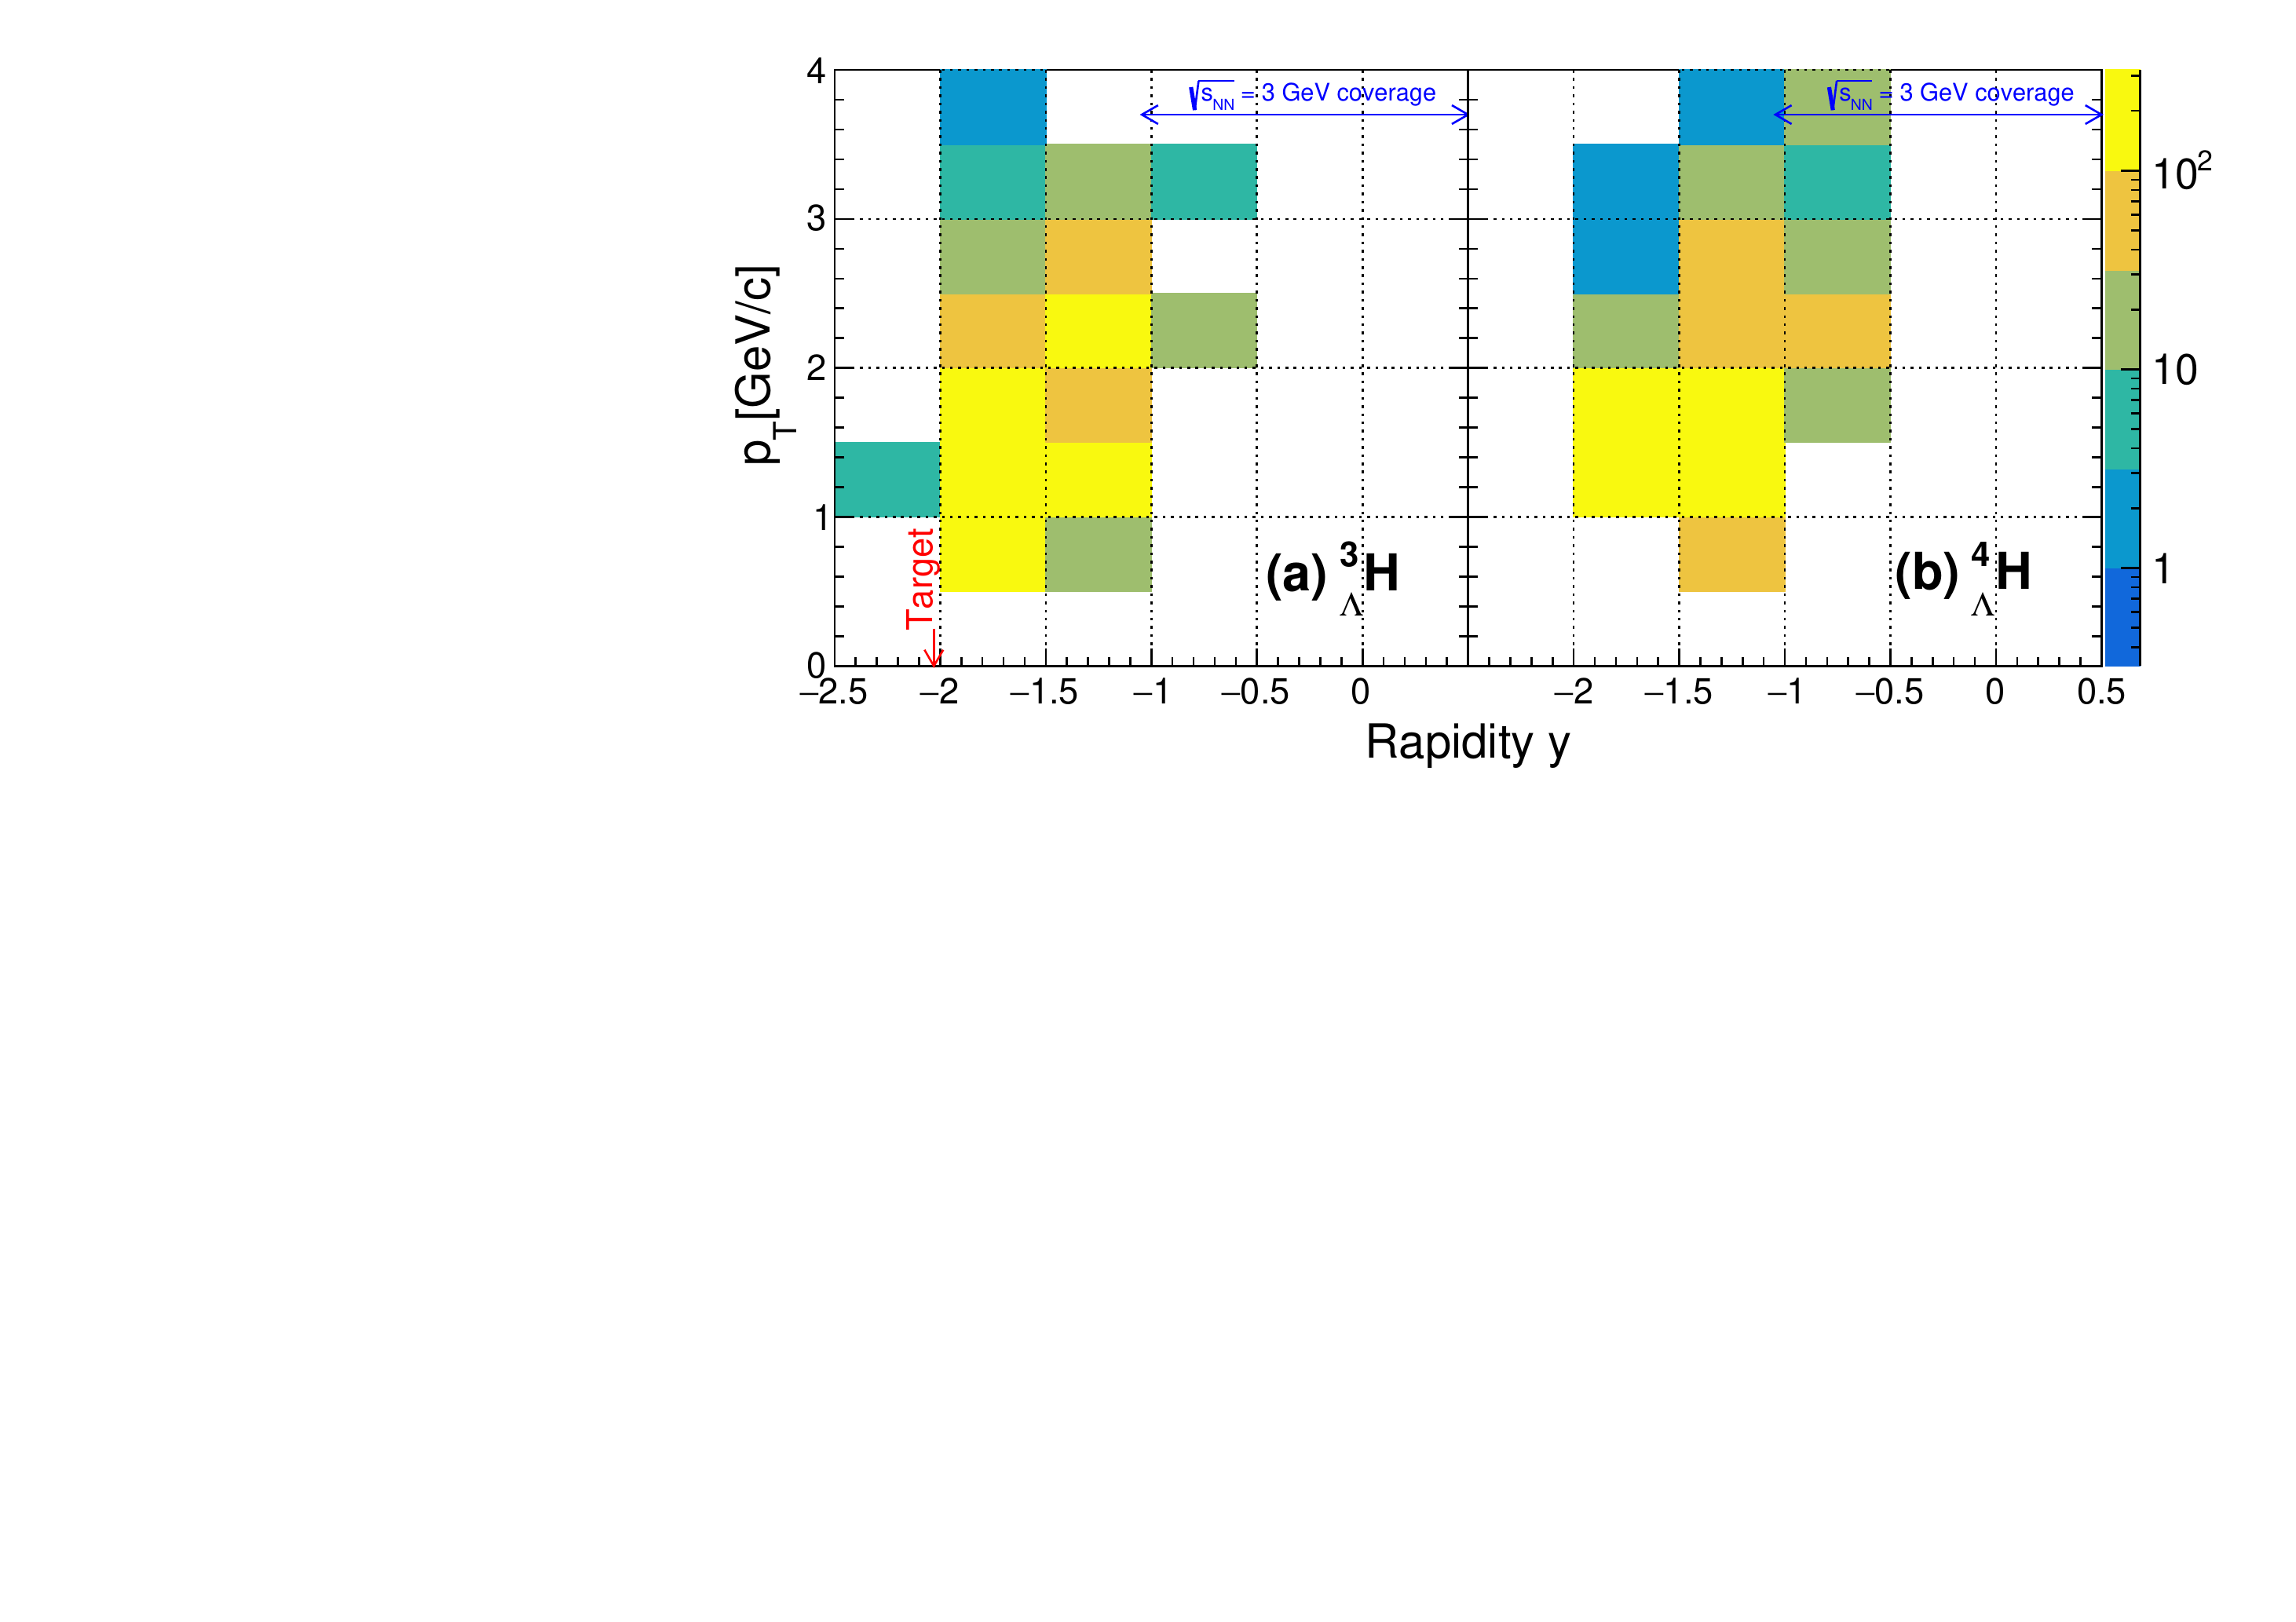}}
\caption{The transverse momentum ($p_{T}$) versus the rapidity (y) for reconstructed (a)\hyt and (b)\hyh. The target is located at the $y = -2.03$.}
\label{fig:7p2acc}
\end{figure}

As in the \snn = 3.0\,GeV analysis, signal counts are extracted as a function of $L/\beta\gamma$ and corrected for efficiency using GEANT simulations. Fig.~\ref{fig:7pslbg} shows the corrected yield normalized by the total yield as a function of $L/\beta\gamma$ for \hyt and \hyh candidates. The yields from the \snn = 3.0\,GeV analysis are shown for comparison. The normalized yields for the two data sets are consistent with each other. 

\begin{figure}[!htb]
\centering
\centerline{\includegraphics[width=0.5\textwidth]{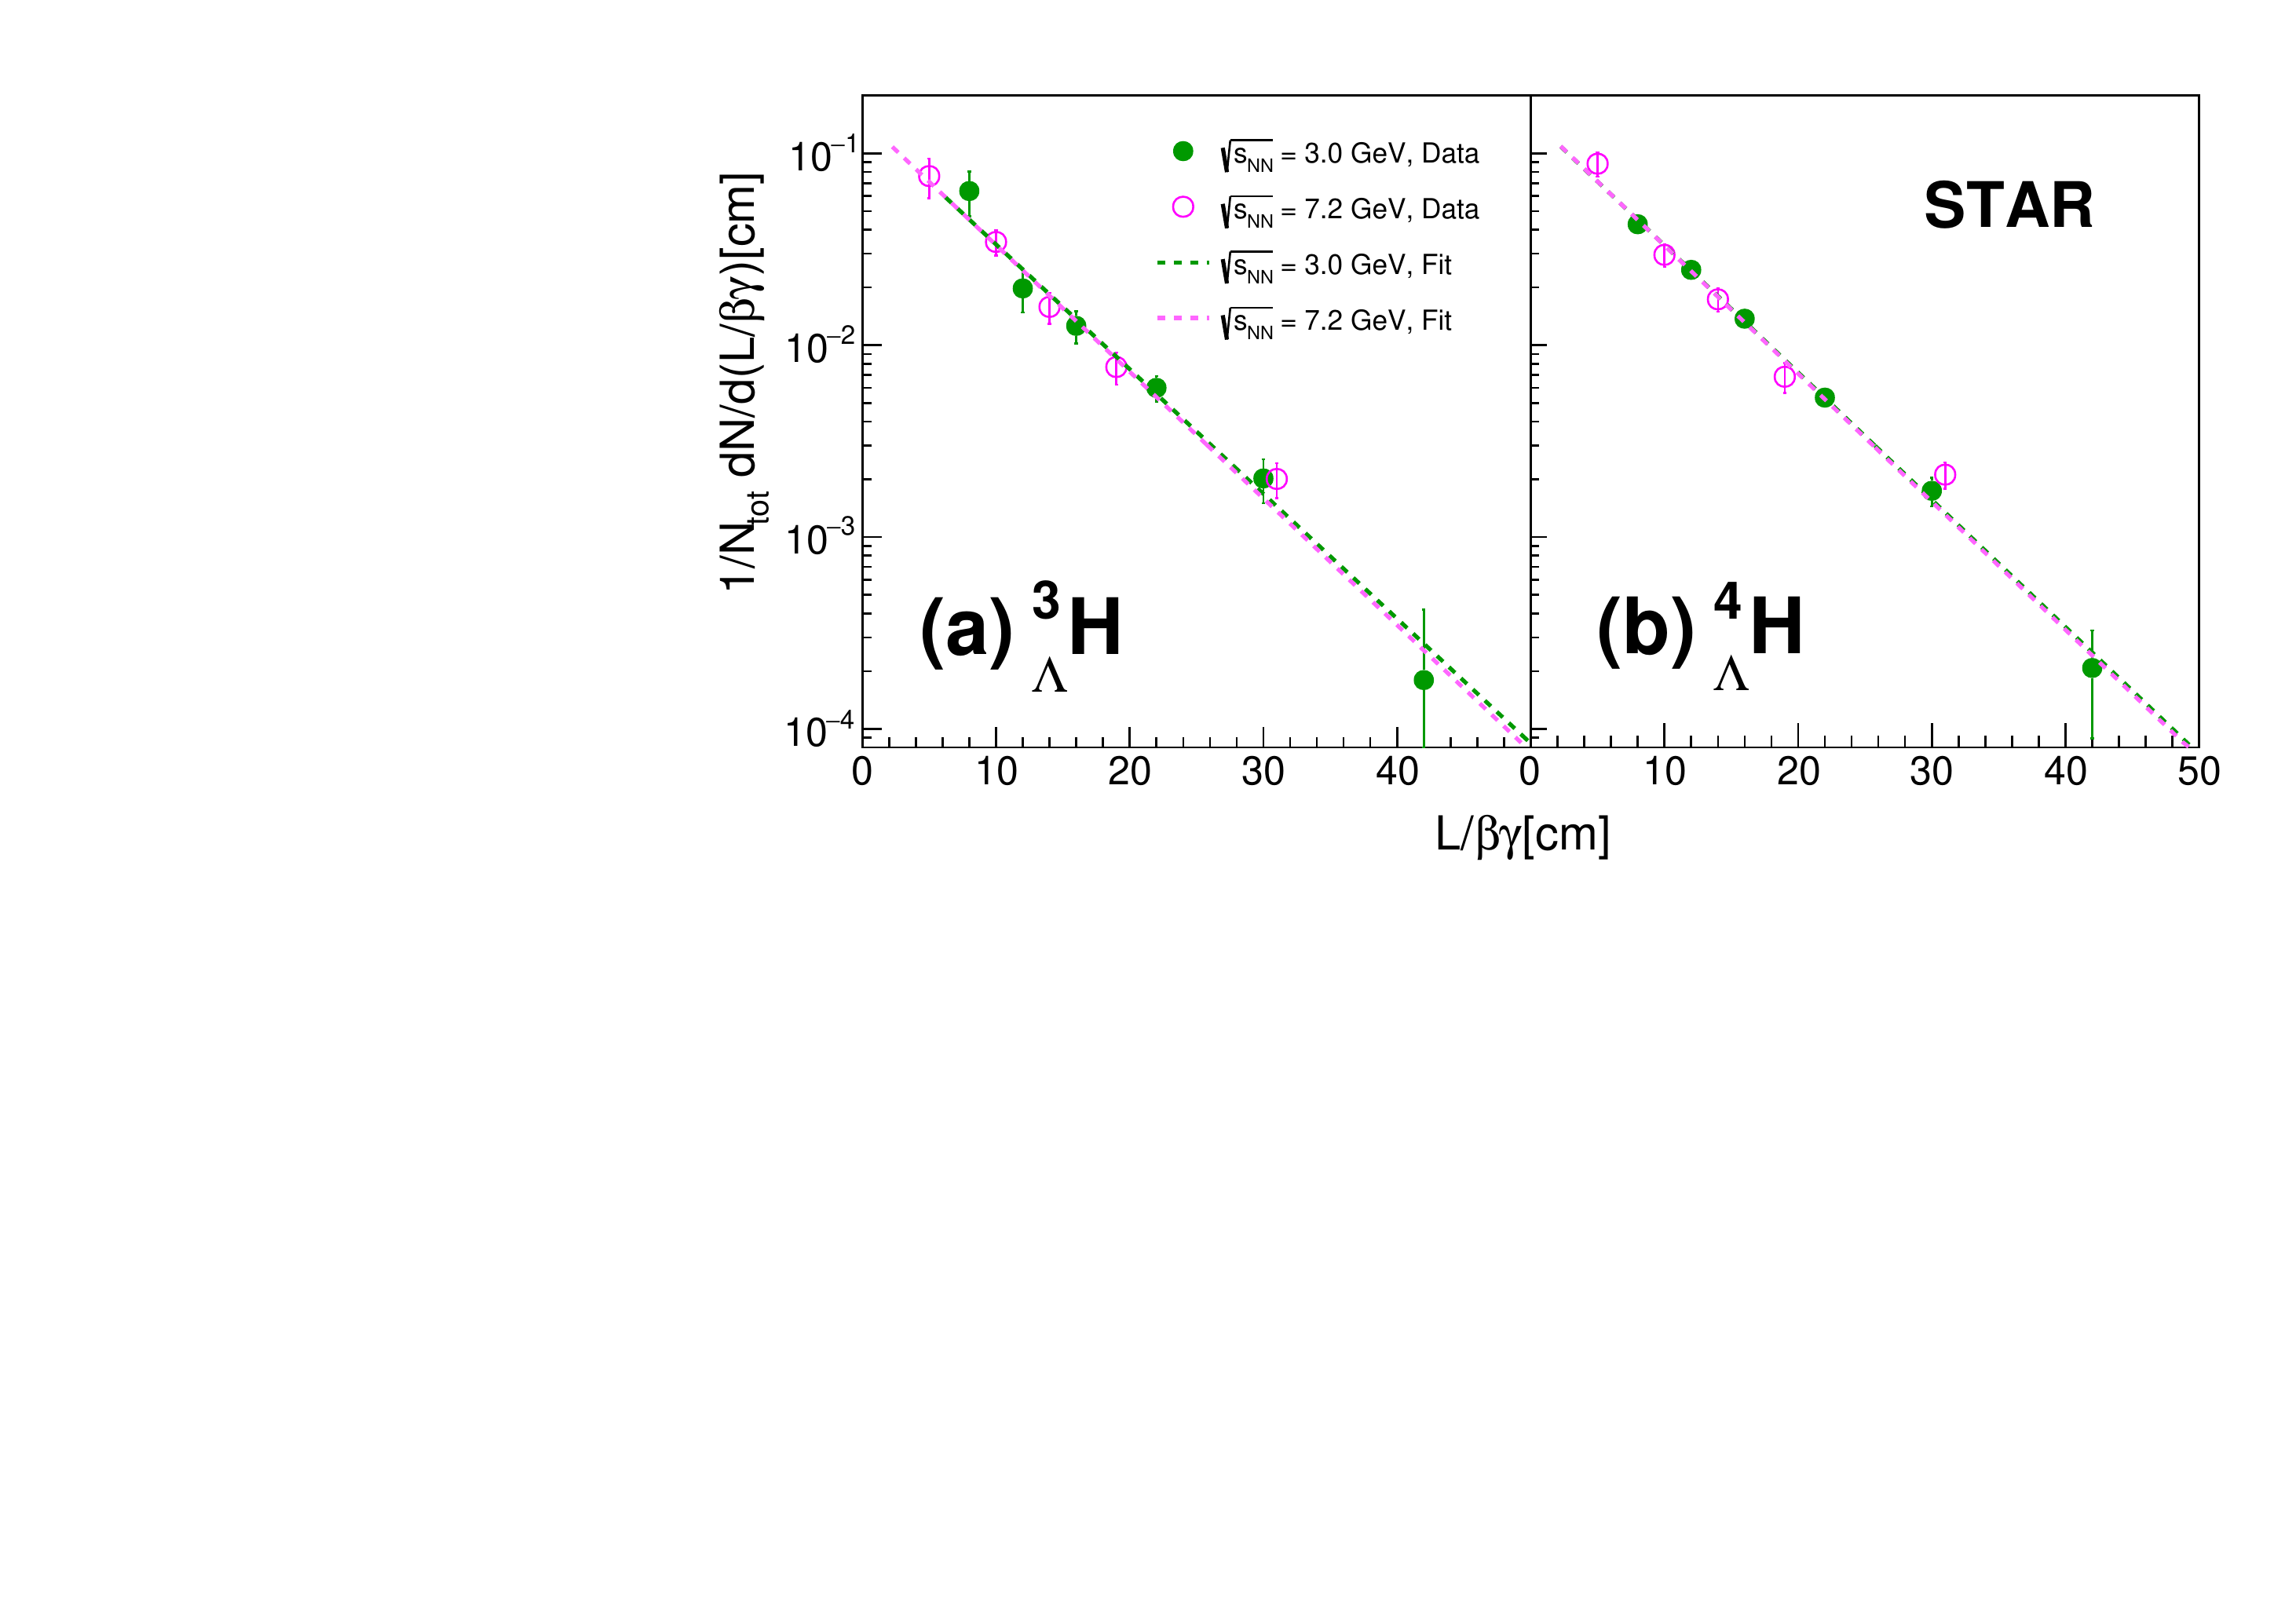}}
\caption{The corrected yield normalized by the total yield versus $L/\beta\gamma$ for (a)\hyt and (b)\hyh. The colored lines represent separate fits to the two data sets.}
\label{fig:7pslbg}
\end{figure}

The yields are fitted with exponential functions to extract the lifetime. The systematic uncertainty analysis for the \snn = 7.2\,GeV data set is identical to that for the \snn = 3.0\,GeV data set, as described in the main text. A breakdown of the systematic uncertainties for \snn = 7.2\,GeV analysis is shown in Table~\ref{tab:sys}. 

\begin{table}[!htbp]
    \centering
    \begin{tabular}{c|cc}
    \hline \hline
    & \multicolumn{2}{c}{Lifetime}  \\
        \textbf{Source%syst. uncertainty
        } & \textbf{$^{3}_{\Lambda}\rm{H}$} & \textbf{$^{4}_{\Lambda}\rm{H}$} 
        \\ \hline
        Analysis cuts & $6.5\%$ & $4.4\%$ 
        \\ %\hline
        Input MC  & $3.4\%$ & $1.2\%$ 
        \\ %\hline
        Tracking efficiency & $2.1\%$ & $1.8\%$
        \\ %\hline
        Signal extraction & $3.8\%$ & $5.4\%$ 
        \\ %\hline
        Detector material & $<1\%$ & $<1\%$ 
        \\ \hline
        \textbf{Total} & \textbf{~~$8.5\%$~~} &  \textbf{~~$7.3\%$~~} 
        \\ \hline \hline
    \end{tabular}
    \caption{Summary of systematic uncertainties for the lifetime measurements using $\sqrt{s_{\rm{NN}}}$ = 7.2\,GeV data.}
    \label{tab:sys}
\end{table}

\iffalse
The lifetimes $223 \pm 23 (\rm stat.) \pm 18 (\rm syst.)$ for \hyt and 
$218 \pm  7 (\rm stat.) \pm 13 (\rm syst.)$ for \hyh are obtained from \snn = 3.0\,GeV data, while the results using the \snn = 7.2\,GeV data are $219 \pm 20 (\rm stat.) \pm 19 (\rm syst.)$ for \hyt and 
$217 \pm  16 (\rm stat.) \pm 16 (\rm syst.)$ for \hyh, consistent with the \snn = 3.0\,GeV results.\fi 
The lifetimes $219 \pm 20 (\rm stat.) \pm 19 (\rm syst.)$ ps for \hyt and 
$217 \pm  16 (\rm stat.) \pm 16 (\rm syst.)$ ps for \hyh are obtained from \snn = 7.2\,GeV data, while the results using the \snn = 3.0\,GeV data are $223 \pm 23 (\rm stat.) \pm 18 (\rm syst.)$ ps for \hyt and $218 \pm  7 (\rm stat.) \pm 13 (\rm syst.)$ ps for \hyh. The two results are consistent with each other. Since hypernuclei lifetimes are intrinsic properties and independent of collision systems, we can combine the results by taking a weighted average $\bar{\tau}$ as follows: 
\begin{align}
    \bar{\tau} &= \frac{\sum_{i} w_i \tau_i}{\sum_{i} w_{i}}, \\
    \sigma_{\bar{\tau},{stat}} &= \frac{1}{\sqrt{\sum_{i} w_i}}, \\
    \sigma_{\bar{\tau},{syst}} &= \frac{\sum_{i} w_i \sigma_{i,syst}}{\sqrt{\sum_{i} w_i}}, \\
\end{align}

\noindent where $\tau_{i}$ is the lifetime measured at energy $i$, $\sigma_{i,stat}$ and $\sigma_{i,syst}$ are the statistical and systematic uncertainties of the individual measurements, and $w_{i}=1/\sigma_{i,stat}^{2}$. Here, we assumed systematic uncertainties are fully correlated between the two measurements. The weighted averages are $221 \pm 15 (\rm stat.) \pm 19 (\rm syst.)$ ps for \hyt and $218 \pm  6 (\rm stat.) \pm 13 (\rm syst.)$ ps for \hyh, as reported in the main text.

\section{Additional information on the $\Lambda$ lifetime analysis}

To ensure the robustness of our \hyt and \hyh lifetime analysis, we carried out the same analysis for the $\Lambda$ hyperon using the \snn = 3.0\,GeV data. As in hypernuclei analysis, signal counts are extracted as a function of $L/\beta\gamma$ and corrected for efficiency using GEANT simulations. The corrected yield normalized by the total yield as a function of $L/\beta\gamma$ is shown in Fig.~\ref{fig:ldpl}. 

\begin{figure}[!htb]
\centering
%\centerline{\includegraphics[width=0.4\textwidth]{figs/ld_pl}}
\centerline{\includegraphics[width=0.4\textwidth]{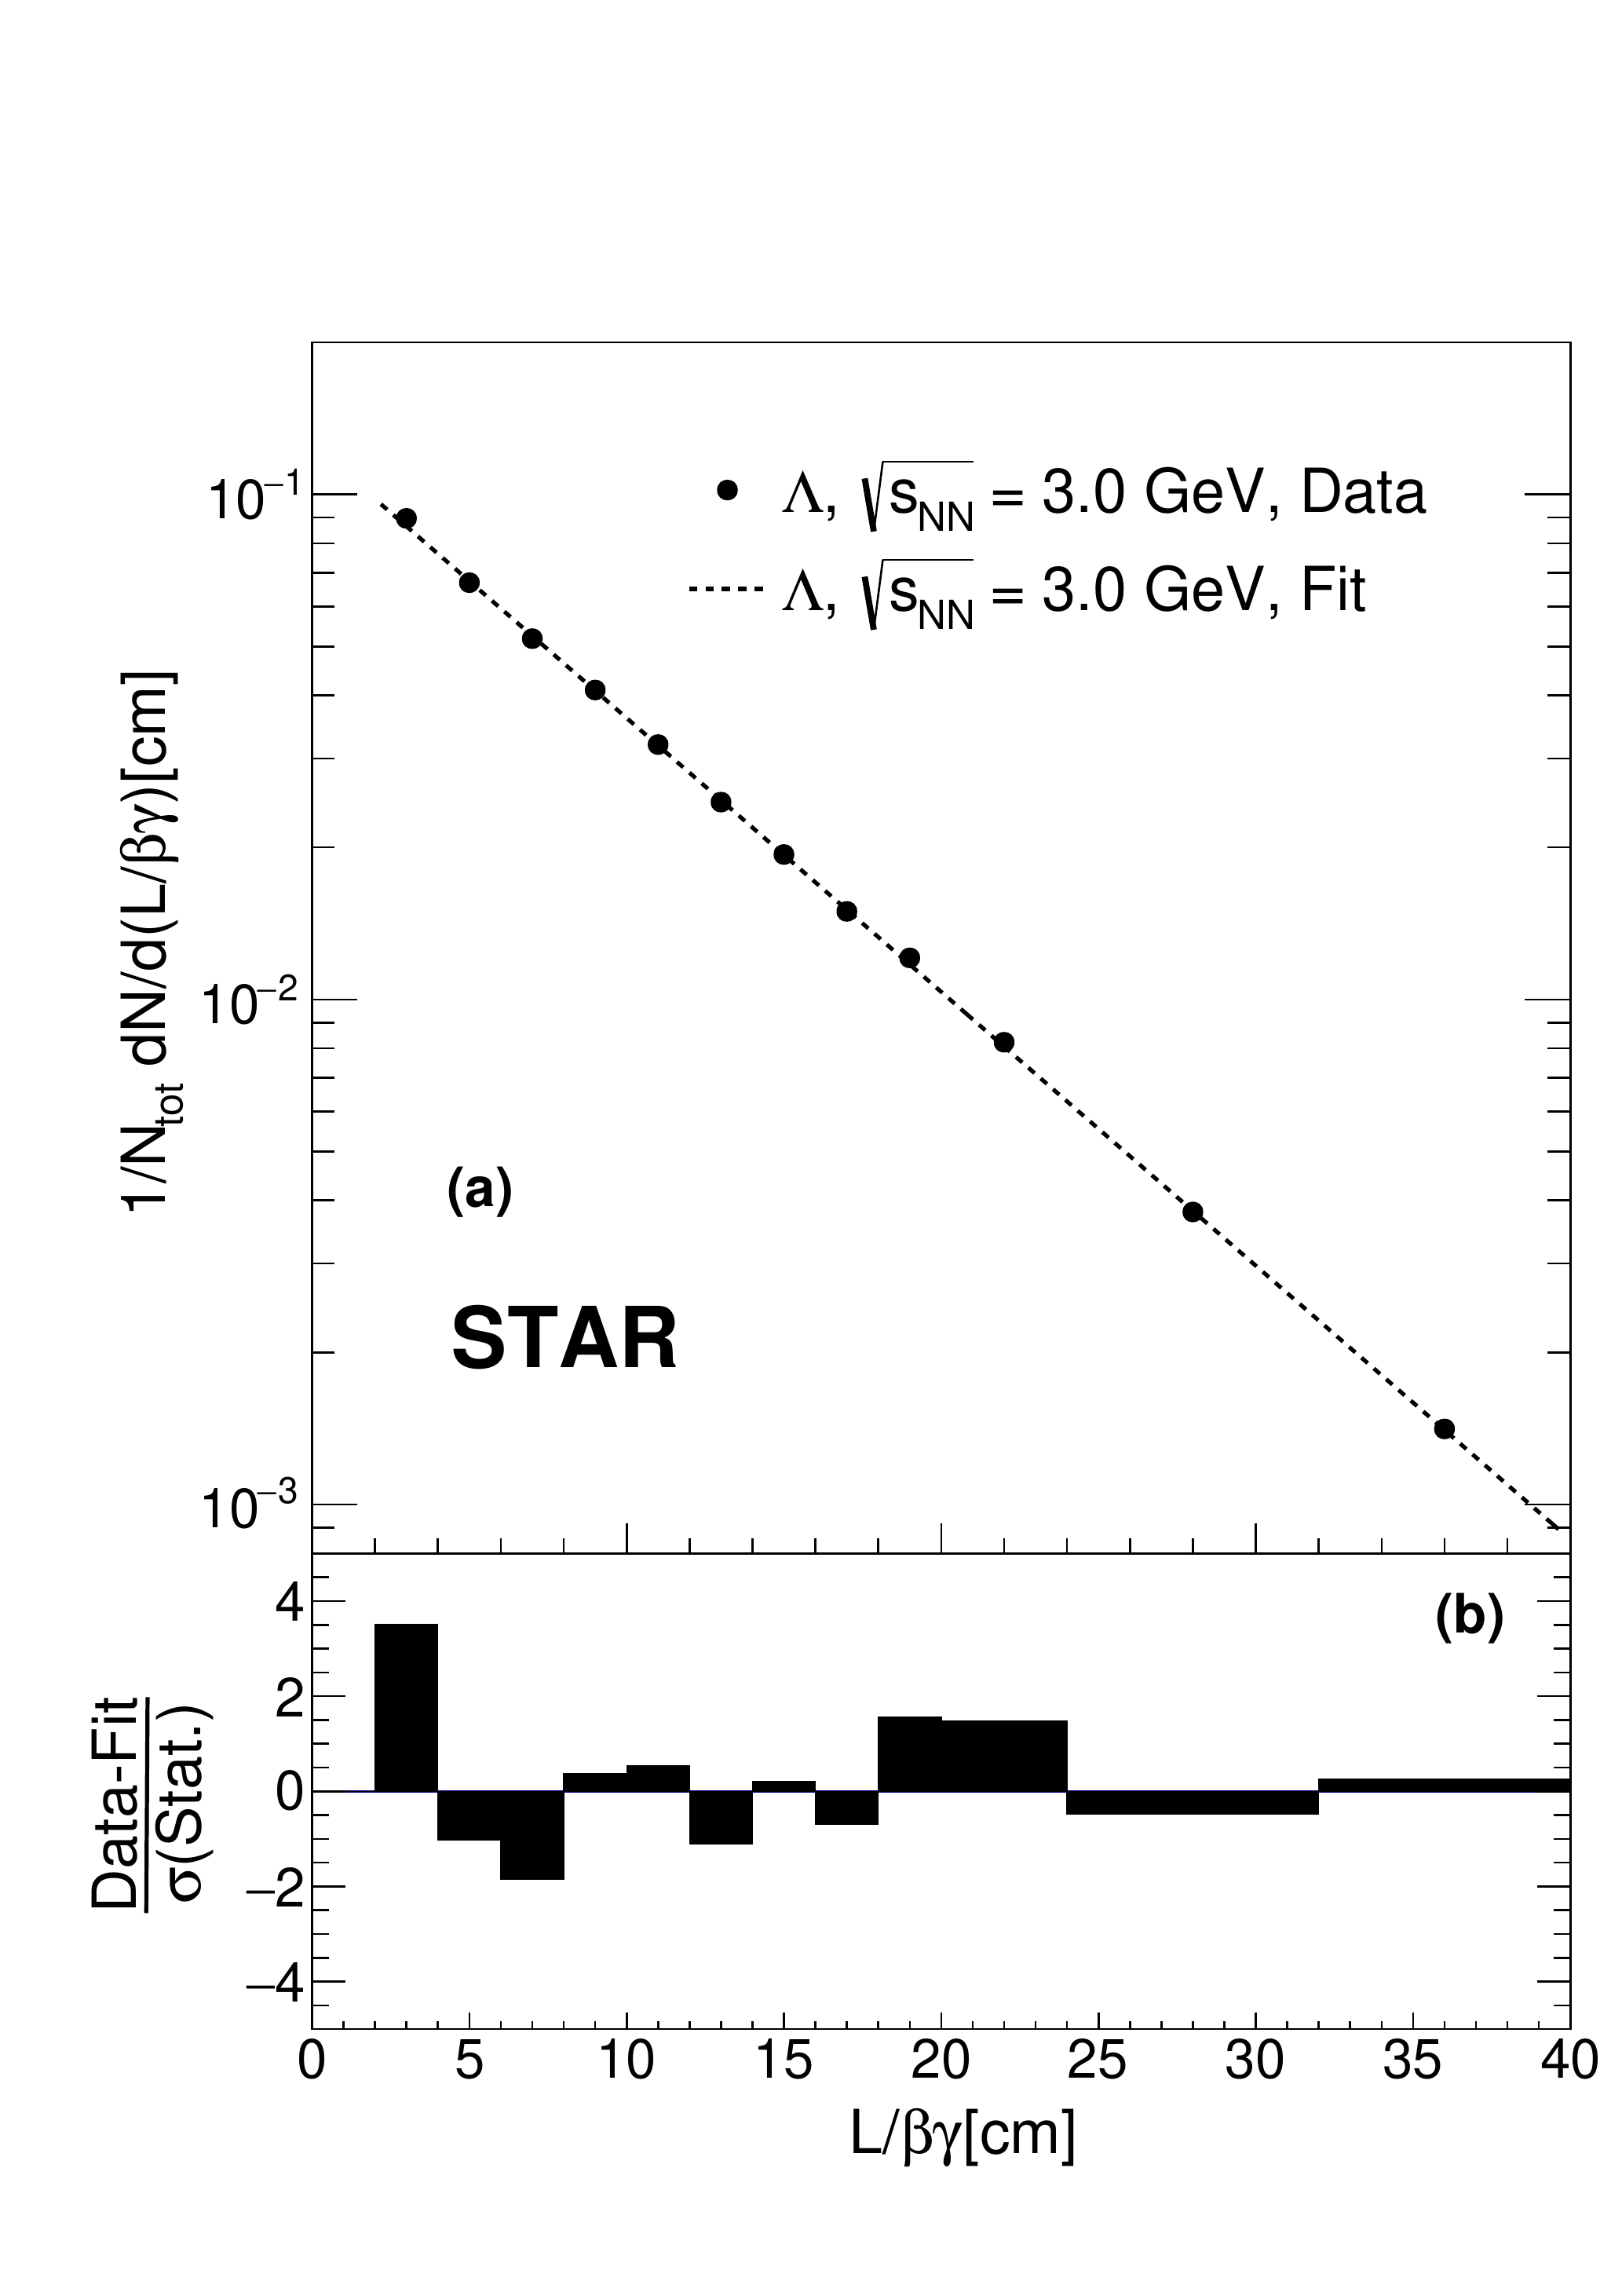}}
\caption{(a) The corrected yield normalized by the total yield versus $L/\beta\gamma$ for $\Lambda$ at $\sqrt{s_{\rm{NN}}}=3$ GeV. The dashed black lines show the exponential fit. (b) Residual distribution of the fit scaled by the statistical uncertainties.}
\label{fig:ldpl}
\end{figure}

The same systematic uncertainties sources considered for hypernuclei analysis are considered for the $\Lambda$ analysis. A breakdown of the systematic  uncertainties is shown in Tab.~\ref{tab:sysld}. The systematic uncertainty on analysis cuts for the $\Lambda$ analysis is smaller compared to the hypernuclei analysis. This is due to two reasons. One, the description of the MC on the number of hits in the TPC is better for protons compared to $^{3}\rm{He}$ or $^{4}\rm{He}$, which may be due to the smaller energy loss in the TPC for protons compared to $^{3}\rm{He}$ or $^{4}\rm{He}$; and two, larger statistical fluctuations in the systematic uncertainty analysis procedure for \hyt and \hyh compared to $\Lambda$.

\begin{table}[!htbp]
    \centering
    \begin{tabular}{c|cc}
    \hline \hline
    & \multicolumn{1}{c}{Lifetime}  \\
        \textbf{Source%syst. uncertainty
        } & \textbf{$\Lambda$} 
        \\ \hline
        Analysis cuts & $0.7\%$
        \\ %\hline
        Input MC  & $1.4\%$
        \\ %\hline
        Tracking efficiency & $0.4\%$
        \\ %\hline
        Signal extraction & $<0.1\%$
        \\ %\hline
        Detector material & $<0.1\%$
        \\ \hline
        \textbf{Total} & \textbf{~~$1.6\%$~~} 
        \\ \hline \hline
    \end{tabular}
    \caption{Summary of systematic uncertainties for the $\Lambda$ lifetime measurement using $\sqrt{s_{\rm{NN}}}$ = 3.0\,GeV data.}
    \label{tab:sysld}
\end{table}

The resulting $\Lambda$ lifetime is $267 \pm  1 (\rm stat.) \pm 4 (\rm syst.)$ ps, consistent with the PDG value~\cite{Zyla:2020zbs}, $263 \pm 2$ ps.

\section{Additional information on centrality definition}

In heavy-ion collisions, the invariant yields of produced particles are highly dependent on the volume of the interacting region, which is related to the impact parameter of the two colliding nuclei. Centrality is a quantity (ranging from $0\%$ to $100\%$) that is introduced to characterize events based on the impact parameter, which is inferred by comparing data and simulations of collisions. Collisions with smaller centrality values are referred to as central events and correspond to smaller impact parameters, while collisions with larger centrality values are referred to as peripheral events and correspond to larger impact parameters. For example, events with $0-10\%$ centrality correspond to the $10\%$ events with the smallest impact parameters. 

The procedure to determine the centrality definition in our analysis follows closely the method as documented in~\cite{STAR:2020dav}. The centrality of each event is characterized by the no. of charged tracks within the TPC acceptance. A Glauber model Monte Carlo method~\cite{STAR:2021hyx} is used to model the collision of two Au nuclei, while a negative binomial distribution is employed to model particle production in hadronic collisions. Model parameters are fitted to the data. Comparison of the Glauber Monte Carlo and the data indicates that the trigger efficiency approaches unity for the most central collisions, and drops to $0.8$ at $60\%$ centrality. We thus restrict our analysis to $0-50\%$ centrality to ensure high trigger efficiency.

\section{Additional information on the \hyt, \hyh $dN/dy$ analysis}
Fig.~\ref{fig:ptspectra} shows the corrected \hyt and \hyh invariant yields as a function of $p_{T}$ for various rapidity ranges in $0-10\%$ and $10-50\%$ centrality Au$+$Au collisions at \snn = 3.0\,GeV. The \hyt and \hyh yields at $y=(-0.5,-0.25)$ and $y=(-0.75,-0.5)$ are scaled by $10^{-1}$ and $10^{-2}$ for visibility. Dashed lines represent fits to the data using the $m_{T}$-exponential function, which are one of the functions used to extrapolate to the unmeasured $p_{T}$ region. 

\begin{figure}[!hb]
\centering
\centerline{\includegraphics[width=0.5\textwidth]{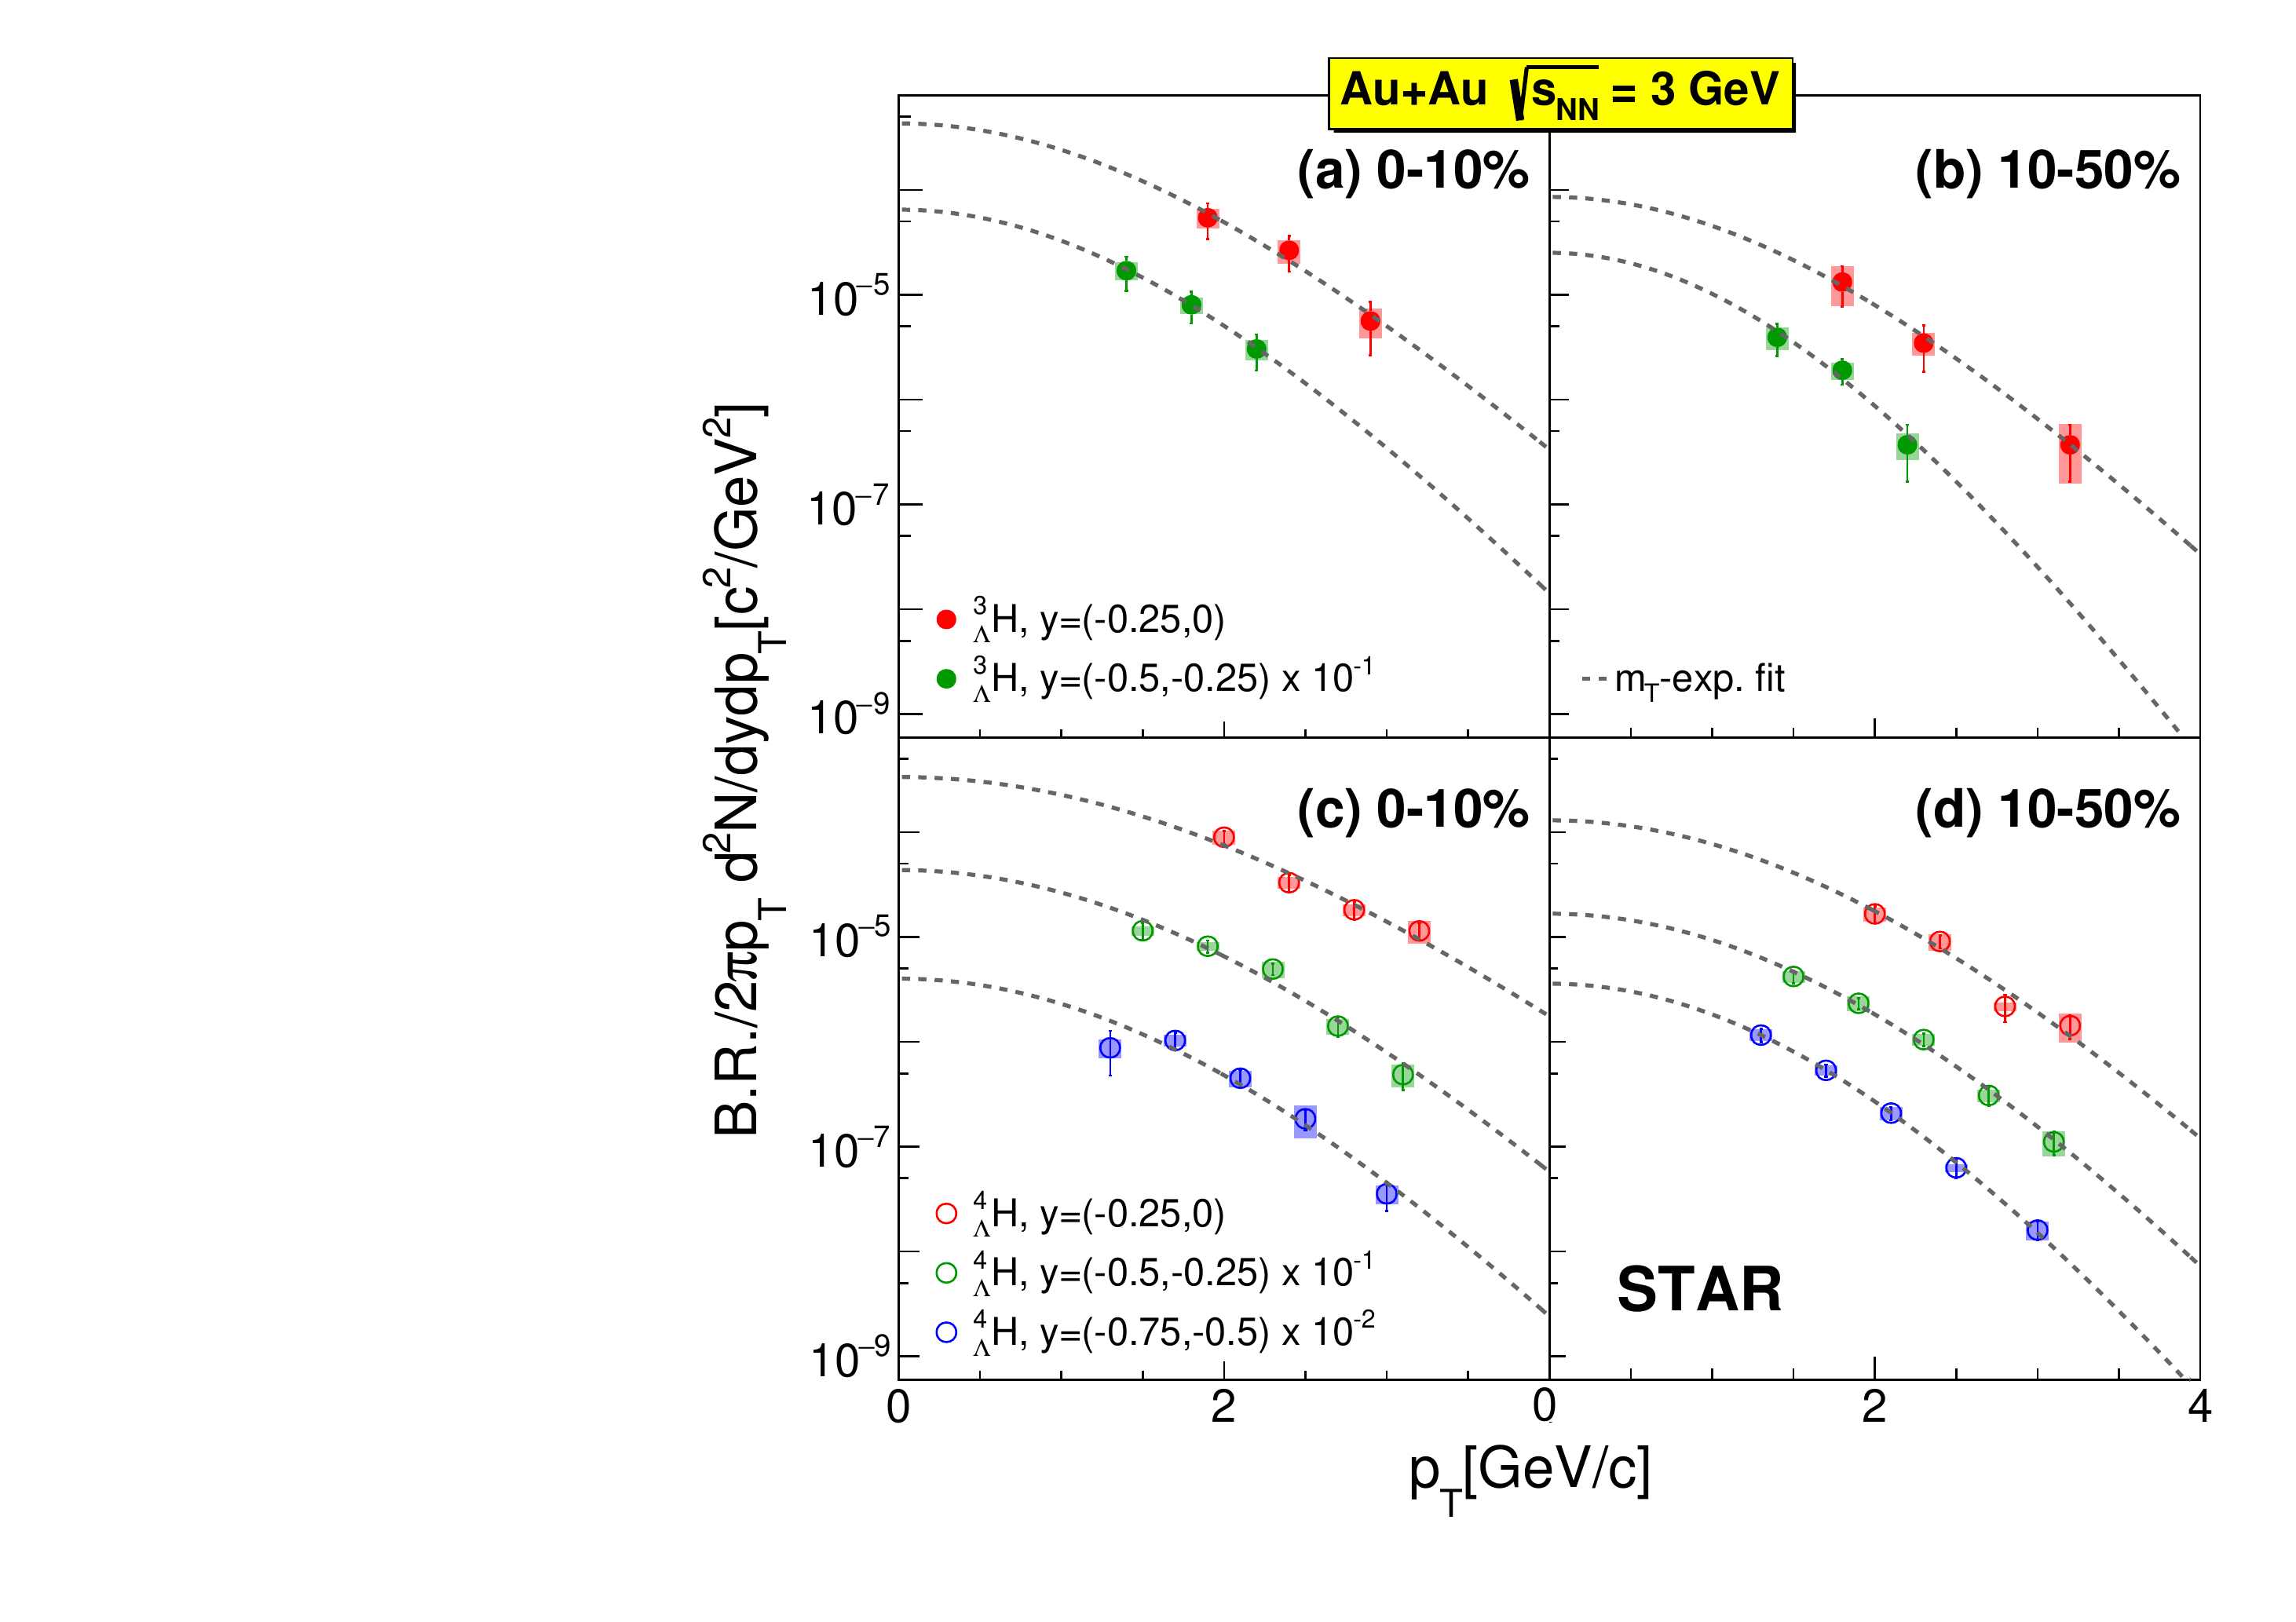}}
\caption{(a)\hyt and (b)\hyh invariant yields as a function of $p_{T}$ for various rapidity regions in $0-10\%$ and $10-50\%$ centrality Au$+$Au collisions at \snn = 3.0\,GeV. Vertical lines represent statistical uncertainties, while boxes represent systematic uncertainties. The dashed black lines represent $m_{T}$-exponential function fits to the measured data points.}
\label{fig:ptspectra}
\end{figure}

To estimate systematic uncertainties, the following functions are considered for extrapolation:

\begin{align}
\begin{split}
    m_{T}-\rm{exponential}&: \frac{dN}{m_{T}dm_{T}} \propto
     \rm{exp}(-m_{T}/T_{m_{T}}),\\
    p_{T}-\rm{Gaussian}&: \frac{dN}{p_{T}dp_{T}} \propto \rm{exp}(-p_{T}^{2}/T_{p_{T}}^{2}),\\
    p_{T}^{1.5}-\rm{exponential}&: \frac{dN}{p_{T}dp_{T}} \propto \rm{exp}(-p_{T}^{1.5}/T_{p_{T}}^{1.5}),\\
    \rm{Boltzmann}&: \frac{dN}{m_{T}dm_{T}} \propto m_{T}\rm{exp}(-m_{T}/T_{B}),\\
    \end{split}
\end{align}

\noindent where $T_{m_{T}}$, $T_{p_{T}}$, and $T_B$ are fit parameters. The $m_{T}$-exponential function is taken to be the default function, and the systematic uncertainty is taken to be the maximum difference between the result using the default function and that using other functions.

\bibliography{supp_reference.bib}
%\end{linenumbers}
\end{document}
